# Supplementary material for: #StayHome or #Marathon? Social Media Enhanced Pandemic Surveillance on Spatial-temporal Dynamic Graphs
Source: arXiv:2108.03670 source file (2021-08-08)
Supplement: Supplementary file 1 [file 6-appendix.tex]

\begin{figure*}[ht]
    \centering
    \includegraphics[width=\linewidth]{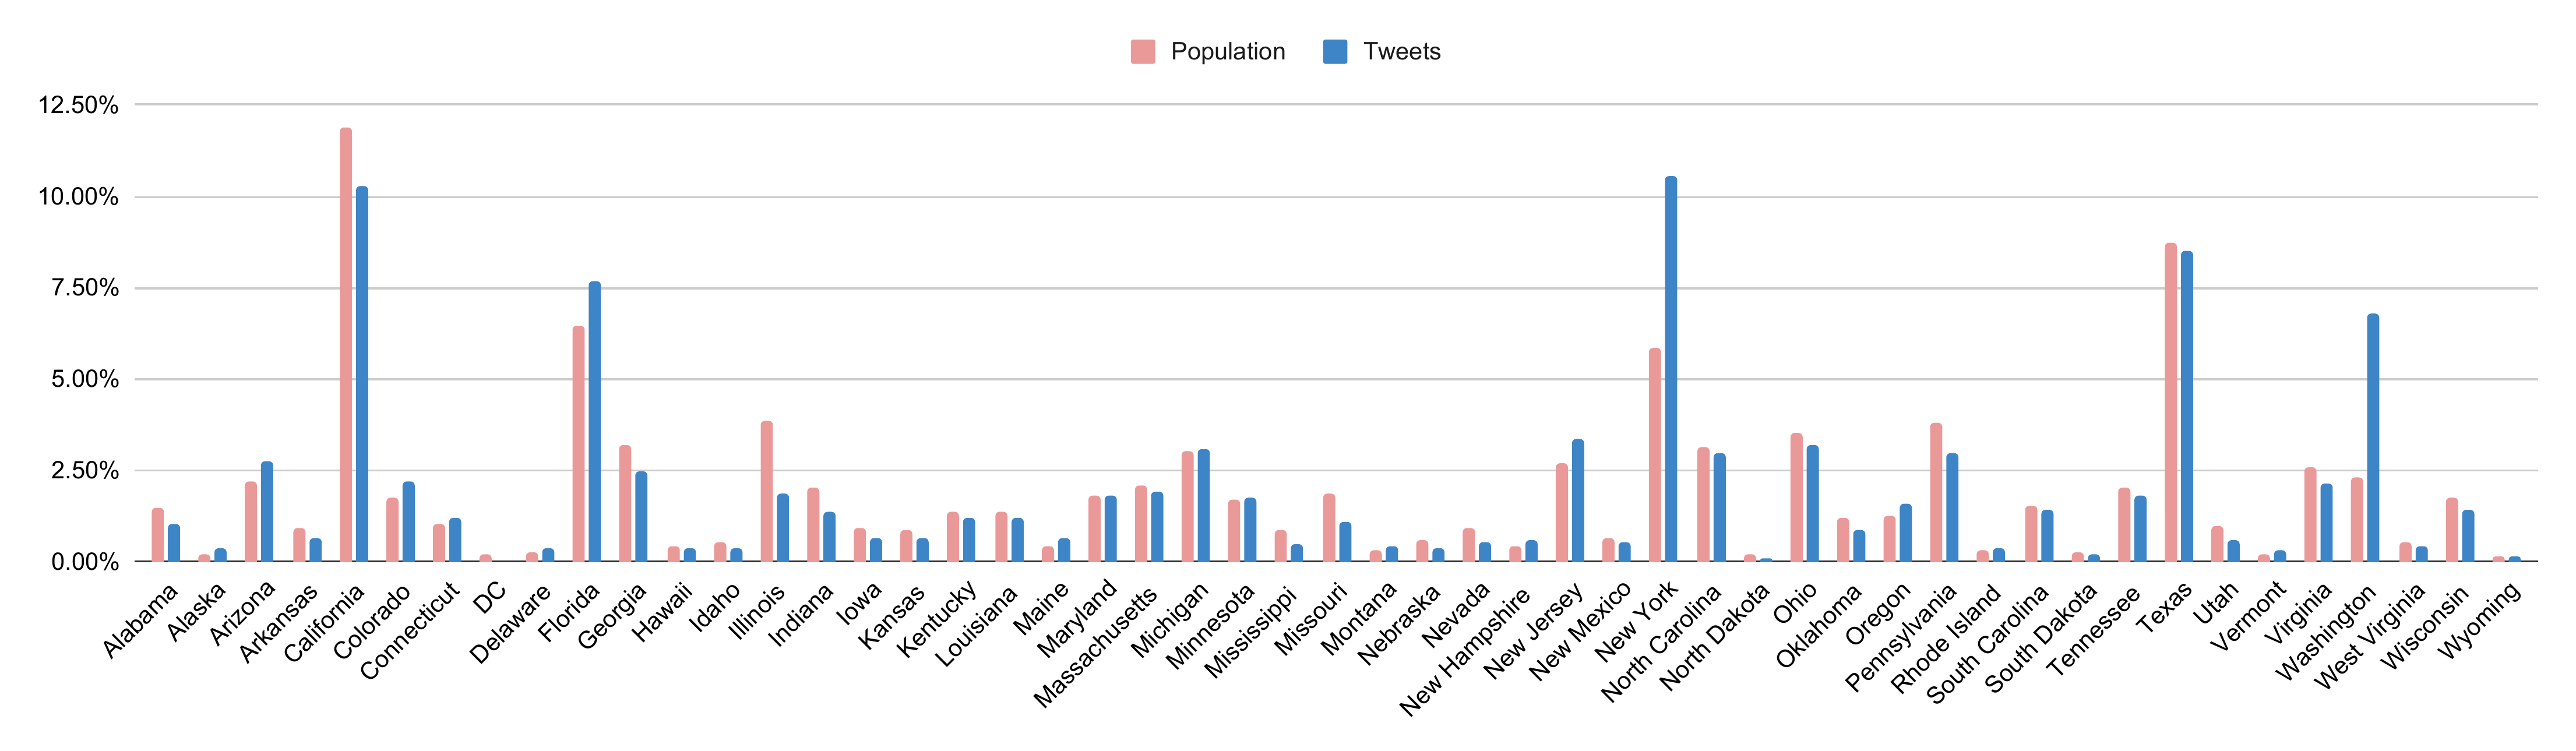}
    \caption{Caption}
    \label{fig:pop}
\end{figure*}
\begin{figure*}[ht]
    \centering
    \includegraphics[width=\linewidth]{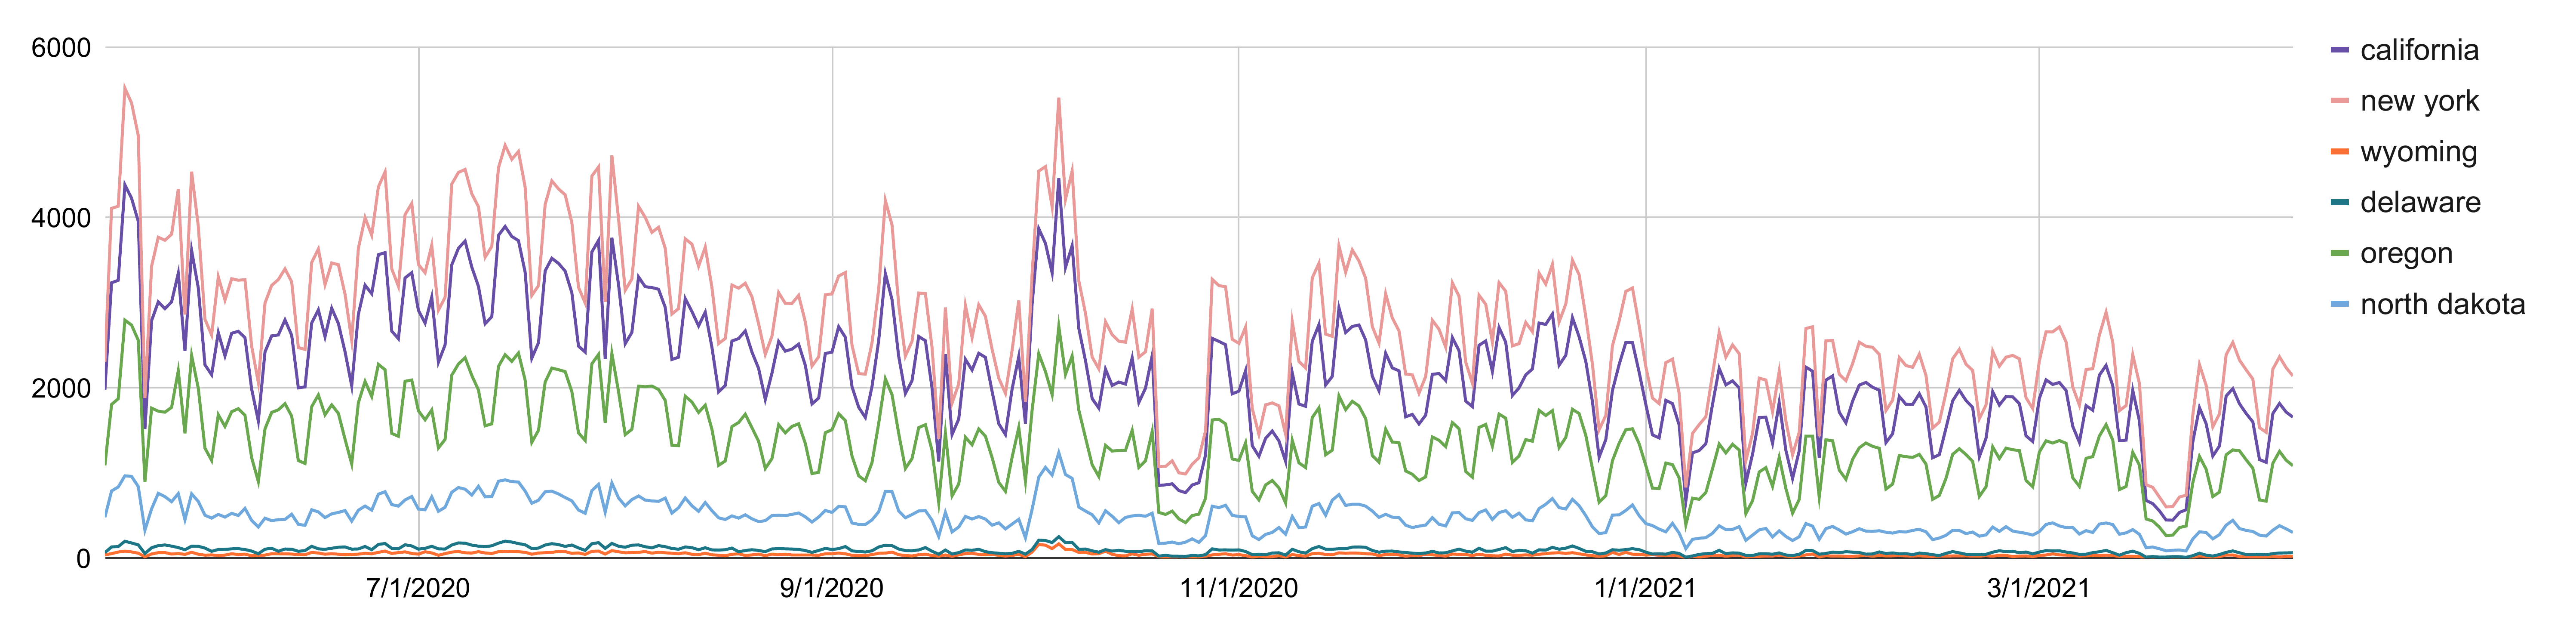}
    \caption{Caption}
    \label{fig:ent}
\end{figure*}

\begin{figure}[ht]
    \centering
    \includegraphics[width=\linewidth]{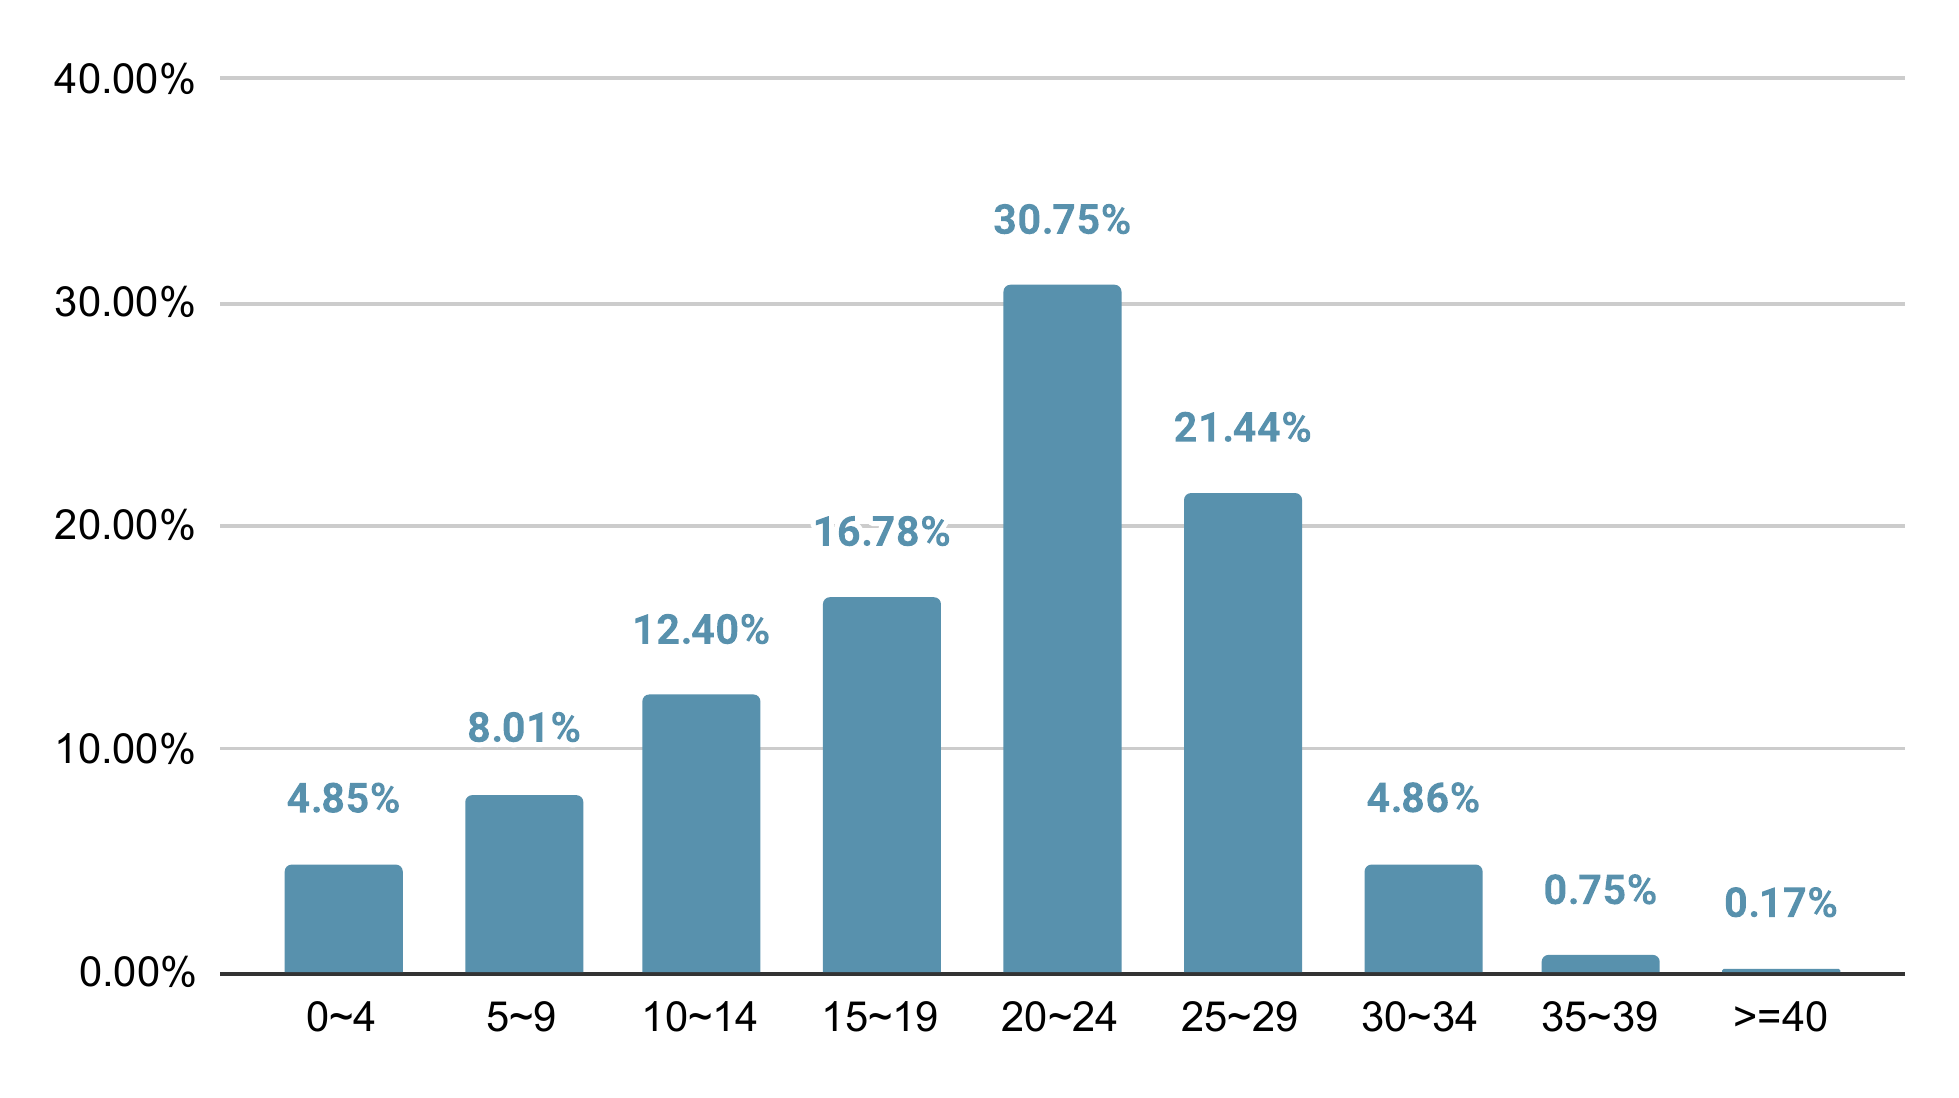}
    \caption{Caption}
    \label{fig:len}
\end{figure}
